# Supplementary material for: The impact of mergers on relaxed X-ray clusters - III. Effects on compact cool cores
Source: arXiv:0804.1552 source file (2008-04-09)
Supplement: Supplementary file 1 [file appendix.tex]

\appendix

\section{An SPH cooling artifact in cluster simulations}\label{appendix-A}

In SPH cluster simulations, cooling converts hot gas in the centre of the system into dense cold gas which is then (when star formation is included) transformed into a collisionless stellar medium.  As a result of the finite timescales involved in transforming cold gas into stars, a multiphase interface forms between dense cold gas and hot rarefied gas at the center.  It is well known that multiphase interfaces of this sort are poorly treated in SPH simulations which incorporate cooling \citep{RT01,MarriWhite03}.  The SPH algorithm computes the volume encompassed by the $N$ nearest neighbours ($N=32$ for our simulations) of a particle and the sum of their masses to form a smoothed density field sampled by each particle.  In regions where there are abrupt density gradients, particles which should be tracing lower density regions can have their densities artificially enhanced due to their proximity to a large number of denser particles.  With the emissivity of the ICM going as $\rho^2$ this can greatly enhance the cooling rate of particles in the core.  In the case of our simulations, this results in a loss of pressure support 3 orders of magnitude in scale as temperatures rapidly drop from $10^7$K to $10^4$K.  With this loss of pressure support, the hot ICM is able to quickly collapse inwards on free-fall timescales which are shorter than the proper cooling timescale.  The result is a quasi-adiabatic flow which drives compressional heating as hot material collects several kernel radii outside of the multiphase interface.  Thus, resolution dependent numerical inaccuracies lead to artificially suppressed densities and enhanced temperatures and entropies in the cores of our systems.  These effects appear initially within a couple smoothing kernel sizes of the multiphase interface at $r\sim 3$\kpc~ but their influence slowly propagates outwards.  To achieve our goal of accurately simulating our clusters at $r>40$\kpc, we must ensure that the influence of this numerical artifact is contained within those radii for the lengths of time that our systems possess dense cores and are actively cooling.

The convergent state of cool core systems such as the ones we have sought to model should involve simple power laws in density and temperature, the logarithmic slope of which are set by the logarithmic slope of the potential (itself a power law for a system gravitationally dominated by an NFW-like dark matter halo) and the temperature dependence of the cooling gas' emissivity.  In Figure \ref{fig-residuals} we present the densities and temperatures of the central regions of a $10^{14.5}\msun~$ system at 1 and 4 \Gyrs~ which we have evolved in isolation.  The results of two runs of differing resolution are illustrated: one at the nominal resolution of the simulations we present in this paper (blue points) and one at $4 \times$ our mass resolution (red points).  We note that after 1 \Gyr~ of evolution, both simulations trace the same power laws in both density and temperature.  After 4 \Gyrs, significant differences within 30\kpc~ have developed.  For both times we have fit power laws to the central density and temperature of the $4\times$ mass resolution runs.  The residuals of subtracting these fits from the particle densities and temperatures of both simulations are illustrated in the lower panels of each case.  From these experiments we see that the nominal resolution runs used for our simulations agree with the results of a significantly higher resolution simulation at an accuracy of 10\% over 4\Gyrs~ for radii beyond our objective of 40 \kpc.

Although this test is run for only $4$\Gyrs~ while our simulations are run for $12$\Gyrs, such numerical concerns are significant only while a core is dense and its cooling timescales very short.  In each of our simulations, the cores of both systems become sufficiently disturbed by the interaction to alleviate this problem.  Periods of active cooling are restricted to durations shorter than $4$\Gyrs, marginalizing concerns regarding over cooling at multiphase interfaces.  Since the effects of the multiphase artifact remain confined to within $40$\kpc~ of the center on those timescales, we thus conclude that we have achieved reasonable resolutions for the requirements of our study.

Although unrelated to the effects of this numerical artifact, we also see in Figure \ref{fig-residuals} a rise in core temperatures within $R_{cool}$.  This is a result of the increasing potential of the core resulting from the migration of baryonic material inwards as cooling converts gas into a pressureless stellar medium.

The effects of this artifact are likely of significant relevance to cosmological simulations.  It has been found that such simulations produce flat entropy cores \citep{Daveetal02} with levels similar to our isolated cluster tests.  Compact cool cores can exist in states of undisturbed cooling for significantly longer durations than in our simulations raising concerns that such entropy floors are a product of numerical effects such as these.
